# Supplementary material for: Band alignment and scattering considerations for enhancing the thermoelectric power factor of complex materials: The case of Co-based half-Heuslers
Source: arXiv:1905.07951 source file (2019-05-20)
Supplement: Supplementary file 1 [file SupplementaryInformation.pdf]

## Supplementary information

### 1. Comparison of the calculated conductivity with experimental data: TiCoSb

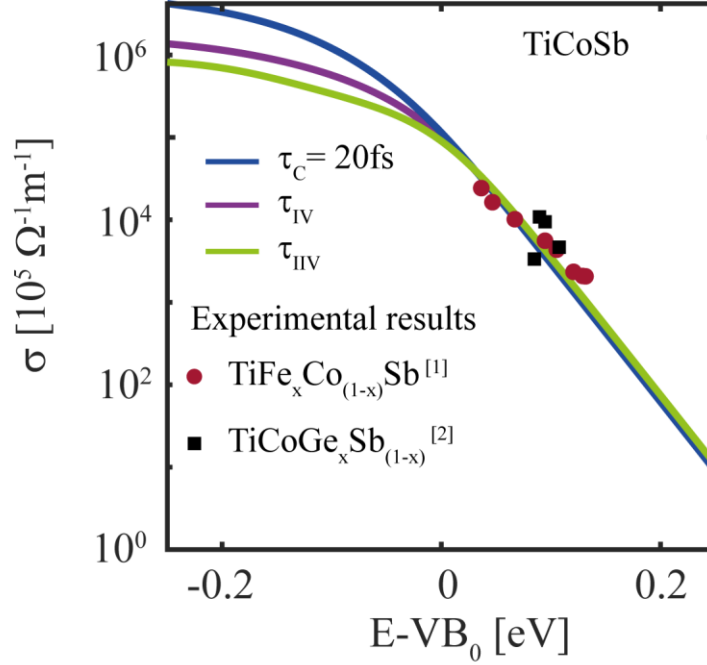

**Figure 1:** Conductivity of TiCoSb calculated under different relaxation time approximations compared with experimental values.

Figure 1 shows the experimental conductivity values versus charge density for 2 TiCoSb alloys, alongside calculated conductivities under different scattering scenarios. The calculated conductivities are for: 1) constant relaxation time –blue line ( $\tau = 20 \text{ fs}$  is used to match experimental values from references [56] and [55]), 2) intra-valley only, purple line and 3) inter- and intra- valley scattering, green line. From the data, one can extract an estimate of a relaxation time, however, lot more information and especially at higher densities are needed to identify the nature of scattering more accurately.

## 2. Electron relaxation through electron-phonon interactions: TiCoSb and ZrCoSb

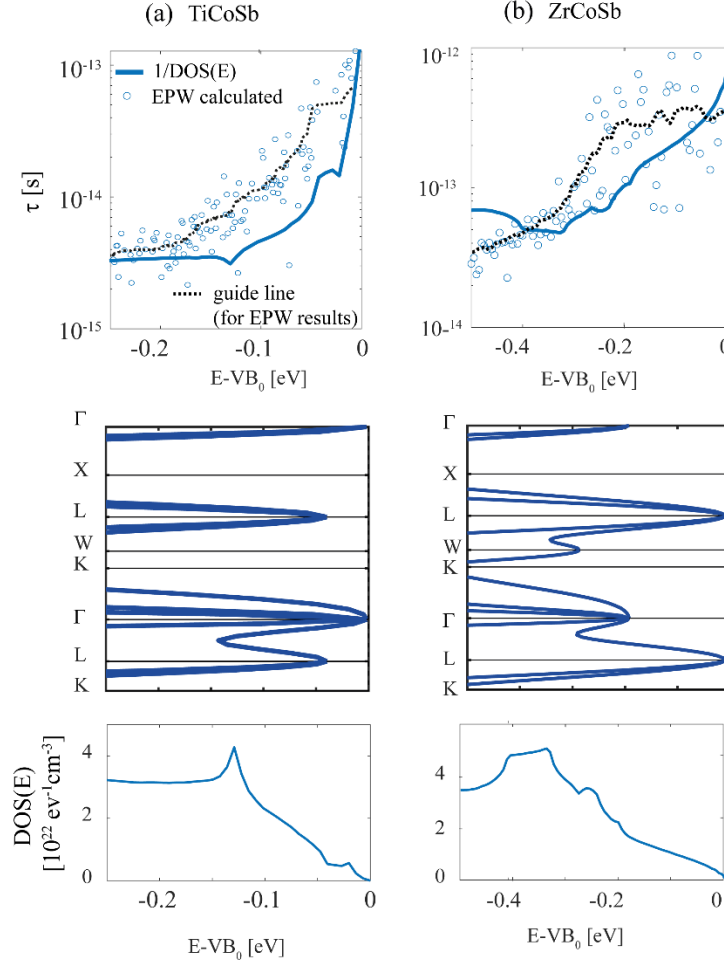

Figure 2 caption: (a-b) Electron relaxation time calculated by considering electron relaxation through EPW electron-phonon interactions (circles-first row), along with the bandstructures (second row) and density of states (third row) for (a) TiCoSb and (b) ZrCoSb. The solid line in (a, b) indicates the trend for  $1/\text{DOS}(E)$ , and the dashed line a guide for the eye fit of the EPW obtained data.

We have calculated the electron-phonon relaxation rates using the electron and phonon bandstructures obtained from *ab-initio* DFT studies for: unstrained TiCoSb and ZrCoSb. The QUANTUM ESPRESSO package was used for bandstructure calculations, and the EPW package<sup>[57]</sup> was used to calculate the relaxation times. Norm-conserving pseudopotentials were used with the PBE-GGA functional and a kinetic energy cutoff greater than 60Ry was used for wavefunctions. An energy convergence criterion of  $10^{-14}$  Ry for self-consistency was adopted throughout our calculations. For electron self-energy calculations, a k-point grid of  $24 \times 24 \times 24$  and a q-point grid of  $4 \times 4 \times 4$  were used for ZrCoSb and a k-point grid of  $18 \times 18 \times 18$  and a q-point grid of  $18 \times 18 \times 18$  were used for TiCoSb. Electron relaxation rates were calculated from the electron self-energy.

The results are shown below in Fig. (2a) and (2b). The circles are the electron-phonon scattering times from EPW, whereas the solid line indicates the  $1/\text{DOS}(E)$  trend (shifted arbitrarily to map the EPW data). The EPW data is quite scattered, having a downward trend. Our intention here is to observe if: 1) the electron-phonon interaction is constant, 2) if it follows  $1/\text{DOS}(E)$ , 3) if there are clear deviations from  $1/\text{DOS}(E)$  in the energies where new bands are encountered. In both materials, one clear observation is that the relaxation time is not a constant and it roughly follows  $1/\text{DOS}(E)$ , with stronger scattering suggested from EPW for energies far away from the band edge. In Fig. 2(c)-(d), and Fig. 2(e)-(f) we show the bandstructures and  $\text{DOS}(E)$ , respectively, for a direct comparison. The  $1/\text{DOS}(E)$  trend, suggests a combined intra- plus inter-valley scattering at first order. On the other hand, large scattering times compared to the  $1/\text{DOS}(E)$  trend, would suggest stronger intra-band scattering. Therefore, to conclude anything on the relative strength of intra- versus inter-valley scattering, a clear deviation in the scattering rates compared to the  $1/\text{DOS}(E)$  needs to be observed when additional bands are encountered. Note, however, that this is a very simplistic picture – in general, the scattering times also depend on the strength of the electron-phonon interactions at different energies, as well as optical phonons that mix different energies. Other than a first order  $1/\text{DOS}(E)$  trend, no other clear evidence can be extracted from the EPW data at this point. (The slope of  $1/\text{DOS}(E)$  in Fig. 2(a) is steeper compared to the EPW results, signalling a possible weaker inter- and intra-valley scattering, but again, concluding confidently would require a lot more work.)

### 3. Bandstructures with spin orbit coupling: TiCoSb, ZrCoSb and NbCoSn

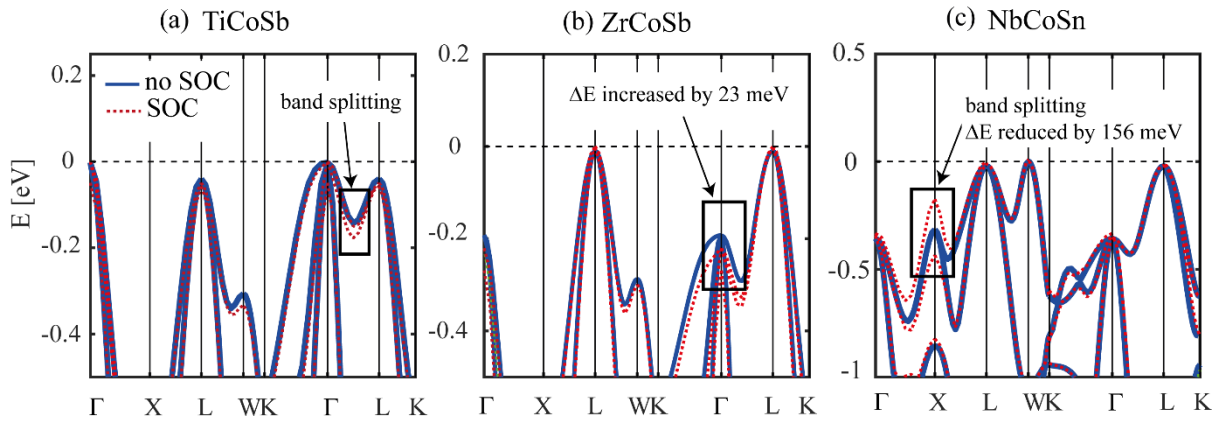

Figure 3 caption: Bandstructures of (a) TiCoSb, (b) ZrCoSb and (c) NbCoSn calculated considering with (solid lines) and without (dotted lines) spin orbit interactions

We have calculated the bandstructures of NbCoSn, TiCoSb and ZrCoSb with spin orbit coupling (SOC) using the QUANTUM ESPRESSO package, employing relativistic pseudopotentials and the PBE exchange-correlation function. The results for the calculation without SOC (blue lines), and with SOC (red lines) are shown in Fig. 3. In the case of the TiCoSb and ZrCoSb in Fig. 3(a) and 3(b), we find that there are no significant effects of SOC at the energies of interest. The works of *Zahedifar et al.*<sup>[50]</sup> and *Zhu et al.*<sup>[53]</sup> state that band splitting and other effects of SOC are smaller than a  $k_B T$  for the light compounds containing Ti and Zr, while they become comparable to  $k_B T$  for the compounds of heavy elements such as Hf. Therefore, reasonable agreement with literature is found here as well.

In the case of NbCoSn in Fig. 3(c), (Nb is heavier than Ti and Zr), our calculations with SOC shows some notifiable effects of band splitting at the X valley and decrease in energy separation between X and L valleys (by 156 meV). This means that valleys can be aligned with less amount of strain, which makes it even more feasible. Under a constant relaxation time, such band splitting would reduce the effectiveness of the band convergence on the power factor, as it reduces the number of carriers contributing near the valence band edge, when the bands are converged. Under energy dependent relaxation times, such splitting can result in either increase or decrease in the power factor, depending on the relative curvature of other bands. However, we do not expect any qualitative alterations to our conclusions, considering that the purpose of this manuscript is to give a qualitative insight into the influence of the band alignment process.
